# Supplementary material for: Networked Restless Multi-Armed Bandits for Mobile Interventions
Source: arXiv:2201.12408 source file (2022-01-28)
Supplement: Supplementary file 1 [file Appendix.tex]

\appendix
\section{Proof of Concavity with Respect to Time Since Last Pull}\label{proof:concav}
In this section, we prove that the reward function of visiting a single location is a monotone increasing concave function with respect the the time elapsed since the arm was last pulled, assuming the initial state is better than the passive steady state ($\frac{s_{0}}{n}> \frac{p^{p}_{BG}}{p^{p}_{GB}+p^{p}_{BG}}$) and no neighboring arms are pulled. We proceed by proving: (1) Given $p^{a}_{v,GB} < p^{p}_{v,GB}$ and $p^{a}_{v,BG}>p^{p}_{v,BG}$ $\forall v \in V$ (intervention assumption 1), we always have $\frac{\hat{p}_{v,BG}}{\hat{p}_{v,GB}+\hat{p}_{v,BG}} > \frac{p^{p}_{v,BG}}{p^{p}_{v,GB}+p^{p}_{v,BG}}$ $\forall v \in V$. (2) Given $\frac{s_t}{n}\geq \frac{p^{p}_{BG}}{p^{p}_{GB}+p^{p}_{BG}}$ and $\frac{\hat{p}_{BG}}{\hat{p}_{GB}+\hat{p}_{BG}} > \frac{p^{p}_{BG}}{p^{p}_{GB}+p^{p}_{BG}}$, pulling the arm will always result in $\frac{s_{t+1}}{n}\geq \frac{p^{p}_{BG}}{p^{p}_{GB}+p^{p}_{BG}}$. (3) For any initial state $\frac{\hat{s}_0}{n}\geq \frac{p^{p}_{BG}}{p^{p}_{GB}+p^{p}_{BG}}$, $(1-p^{p}_{GB}- p^{p}_{BG})>0$ and $\hat{p}_{BG}+\hat{p}_{GB}-p^{p}_{BG}-p^{p}_{GB}>0$ (intervention assumption 2 and 3), the reward function is a monotone increasing concave function with respect to the time elapsed since the last pull. 

We start by proving the first assertion: given $p^{a}_{v,GB} < p^{p}_{v,GB}$ and $p^{a}_{v,BG}>p^{p}_{v,BG}$, by our assumptions, we know that
%\dk{Notice that you are now omitting the commas between $v$ and $BG$ in the subscript. Make sure that this is consistent throughout the paper, including appendices.}
$\hat{p}_{v,GB}=\hat{w}_v p^{a}_{v,GB}+(1-\hat{w}_v) p^{p}_{v,GB}$ for some $0\leq \hat{w}_v \leq 1$ for any action taken. Thus we have $\hat{p}_{v,GB} < p^{p}_{v,GB}$ and $\hat{p}_{v,BG}>p^{p}_{v,BG}$. By rearranging the inequalities by
\begin{align*}
&\hat{p}_{v,BG} \cdot p^{p}_{v,GB} + \hat{p}_{v,BG} \cdot p^{p}_{v,BG} > p^{p}_{v,BG} \cdot \hat{p}_{v,GB} + \hat{p}_{v,BG} \cdot p^{p}_{v,BG},
\end{align*}
we obtain the conclusion (1):
\begin{align*}
&\frac{\hat{p}_{v,BG}}{\hat{p}_{v,GB}+\hat{p}_{v,BG}} > \frac{p^{p}_{v,BG}}{p^{p}_{v,GB}+p^{p}_{v,BG}}.
\end{align*}
%\dk{What do the two preceding inequalities have to do with each other? Please explain, e.g., say that the second is obtained from the first by rearranging, or whatever else is happening. Two inequalities in a row is not helpful.}

%\dk{Delete ``Now''? Change to ``Now, given''? Something else?}
Now, given $\frac{s_t}{n}$, the state after pulling the arm can be calculated as:
\begin{align*}
\frac{s_{t+1}}{n}=(1-\hat{p}_{GB})\frac{s_{t}}{n}+\hat{p}_{BG}(1-\frac{s_t}{n}).
\end{align*}
If $\frac{s_{t}}{n}\leq \frac{\hat{p}_{BG}}{\hat{p}_{GB}+\hat{p}_{BG}}$, we have:
\begin{align*}
(\hat{p}_{GB}+\hat{p}_{BG}+1-1)\frac{s_t}{n}\leq \hat{p}_{BG}
\end{align*}
We can move some of the terms from the left to the right and obtain:
\begin{align*}
\frac{s_t}{n}\leq (1-\hat{p}_{GB})\frac{s_{t}}{n}+\hat{p}_{BG}(1-\frac{s_t}{n})=\frac{s_{t+1}}{n}
\end{align*}
Combining this with the condition $\frac{s_t}{n}\geq \frac{p^{p}_{BG}}{p^{p}_{GB}+p^{p}_{BG}}$, we get:
\begin{align*}
\frac{p^{p}_{BG}}{p^{p}_{GB}+p^{p}_{GB}} \leq \frac{s_t}{n} \leq \frac{s_{t+1}}{n}.
\end{align*}
%\dk{Again, in the preceding, we have a bunch of inequalities, but no discussion what they have to do with each other, how one is obtained from the other, etc. Please elaborate.}

If $\frac{s_{t}}{n} > \frac{\hat{p}_{BG}}{\hat{p}_{GB}+\hat{p}_{BG}}$, using $(1-\hat{p}_{GB}-\hat{p}_{BG})>0$ (see intervention assumption 2) we have:
\begin{align*}
\frac{s_{t+1}}{n} &= (1-\hat{p}_{GB})\frac{s_{t}}{n}+\hat{p}_{BG}(1-\frac{s_t}{n})\\
&> (1-\hat{p}_{GB})\frac{\hat{p}_{BG}}{\hat{p}_{GB}+\hat{p}_{BG}}+\hat{p}_{BG}(1-\frac{\hat{p}_{BG}}{\hat{p}_{GB}+\hat{p}_{BG}})\\
&=\hat{p}_{BG}+(1-\hat{p}_{BG}-\hat{p}_{GB})\frac{\hat{p}_{BG}}{\hat{p}_{GB}+\hat{p}_{BG}}\\
&=(\hat{p}_{BG}+\hat{p}_{GB})\frac{\hat{p}_{BG}}{\hat{p}_{GB}+\hat{p}_{BG}}+(1-\hat{p}_{BG}-\hat{p}_{GB})\frac{\hat{p}_{BG}}{\hat{p}_{GB}+\hat{p}_{BG}}\\
&= \frac{\hat{p}_{BG}}{\hat{p}_{GB}+\hat{p}_{BG}} \\
%&\rightarrow \frac{s_{t+1}}{n} > \frac{\hat{p}_{BG}}{\hat{p}_{GB}+\hat{p}_{BG}} 
&> \frac{p^{p}_{BG}}{p^{p}_{GB}+p^{p}_{BG}},
\end{align*}
which proves (2).
% \dk{Notice that I removed an unnecessary implication by commenting it out.}

Finally, let $\frac{\hat{s}_{\tau}}{n}$ denote the fraction of individuals in the good state $\tau$ steps after an arm pull, and let $\frac{\hat{s}_{0}}{n}$ be its initial state. The reward function $H(\tau,\hat{w})$, where $\tau$ is the time since the last arm pull and $\hat{w}$ the share of the population exposed to an intervention, can be calculated as:
\begin{align*}
H(\tau,\hat{w})=&(p^{p}_{GB}-\hat{p}_{GB})n\hat{w}\frac{\hat{s}_{\tau}}{n}+(\hat{p}_{BG}-p^{p}_{BG})n\hat{w}(1-\frac{\hat{s}_{\tau}}{n})\\
&=(\hat{p}_{BG}-p^{p}_{BG})\hat{w}n-(\hat{p}_{BG}+\hat{p}_{GB}-p^{p}_{BG}-p^{p}_{GB})\hat{w}n\frac{\hat{s}_{\tau}}{n}
\end{align*}
The only variable here is $\frac{\hat{s}_{\tau}}{n}$ with a negative sign and positive coefficient $(\hat{p}_{BG}+\hat{p}_{GB}-p^{p}_{BG}-p^{p}_{GB})\hat{w}n$ (from intervention assumption 3). It is sufficient to prove that $\frac{\hat{s}_{\tau}}{n}$ is a monotone decreasing convex function. Given $\frac{\hat{s}_{0}}{n}$, using an eigendecomposition of the matrix $\mathbf{P}^{p}$, it can be written as:
\begin{align*}
\frac{\hat{s}_{\tau}}{n}=\frac{p^{p}_{BG}}{p^{p}_{GB}+p^{p}_{BG}}+(1-p^{p}_{BG}-p^{p}_{GB})^\tau \cdot
\left(\frac{\hat{s}_{0}}{n}-\frac{p^{p}_{BG}}{p^{p}_{GB}+p^{p}_{BG}} \right),
\end{align*}
which is a monotone decreasing convex function given the intervention assumption 2 (which states that $(1-p^{p}_{BG}-p^{p}_{GB})>0$). This proves the third assertion, and the theorem follows.

\section{Proof of Concavity with Respect to the expected Share of the Population reached by an intervention} \label{proof:portion}
Consider two intervention schedules $\pi_1$ and $\pi_2$, whose respective intervention shares are given by $(\hat{w}_1(\pi_1),\hat{w}_2(\pi_1), \ldots, \hat{w}_T(\pi_1))$ and $(\hat{w}_1(\pi_2),\hat{w}_2(\pi_2), \ldots, \hat{w}_T(\pi_2))$. 
Given $\hat{w}_1(\pi_1)-\hat{w}_1(\pi_2)=\Delta w >0$ and $\hat{w}_t(\pi_1)=\hat{w}_t(\pi_2)$ for all $t>0$, we want to prove that $\pi_1$ always results in higher reward, assuming the same initial state of the node $\frac{s_{0}}{n}$. The total reward gain from one location can be written as
\[
R(\pi)=\sum_{t=0}^{T}(p^{p}_{GB}-\hat{p}_{GB}(\pi))s_{t}(\pi)+(\hat{p}_{BG}(\pi)-p^{p}_{BG})(n-s_{t}(\pi)).
\]
The difference between the rewards of the two policies can thus be calculated as:
\begin{align*}
R(\pi_1)-R(\pi_2)= \Delta w \left( (p^{a}_{BG}-p^{a}_{GB})-(p^{p}_{BG}-p^{p}_{GB}) \right) s_{0}\\
+\sum_{t=1}^{T} \left( (\hat{p}_{BG}(\pi)-\hat{p}_{GB}(\pi)) - (p^{p}_{BG}-p^{p}_{GB}) \right) \Delta s_{t};
\end{align*}
here, $\Delta s_{t}$ denotes the difference between the states induced by the two policies at time $t$. Let $\Delta \mathbf{b}_0=[\Delta w s_{0},-\Delta w s_{0}]^{\top}$, The $\Delta s_{t}$ in each time step can be calculated as:%\dk{I don't see how this parses. You define $\Delta \mathbf{b}_0$, and then write something in the same sentence. Does it follow? How? What do these have to do with each other?}
\[
\Delta s_{t}= [1,0] \prod_{\tau=0}^{t-1}\hat{\mathbf{P}}\Delta \mathbf{b}_0.
\]
Observe that $\mathbf{b}_0$ happens to be an eigenvector of any $\hat{\mathbf{P}}$ with corresponding eigenvalue $(1-\hat{p}_{GB}(\pi)-\hat{p}_{BG}(\pi))$. We have 
\[
\Delta s_{t}=\prod_{\tau=0}^{t-1}(1-\hat{p}_{GB}(\pi)-\hat{p}_{BG}(\pi))\Delta w s_{0}.
\]
From intervention assumption 3, we can infer that $(1-p^{p}_{GB}-p^{p}_{BG})>(1-\hat{p}_{GB}(\pi)-\hat{p}_{BG}(\pi))$. From intervention assumption 1, we can also infer that $p^{a}_{GB}-p^{a}_{BG}>\hat{p}_{GB}(\pi)-\hat{p}_{BG}(\pi)$ at any time step. Combining the above, we can infer that 
\begin{align*}
&R(\pi_1)-R(\pi_2)=\Delta w \left( (p^{a}_{BG}-p^{a}_{GB})-(p^{p}_{BG}-p^{p}_{GB}) \right) s_{0}\\
&-\sum_{t=1}^{T} \left( (\hat{p}_{BG}(\pi)+\hat{p}_{GB}(\pi))-(p^{p}_{BG}+p^{p}_{GB}) \right) \Delta s_{t}\\
&>\Delta ws_{0} \Big[ (p^{a}_{BG}-p^{a}_{GB})-(p^{p}_{BG}-p^{p}_{GB}) \\
&-\sum_{t=1}^{\infty} \left( (\hat{p}_{BG}(\pi)+\hat{p}_{GB}(\pi))-(p^{p}_{BG}+p^{p}_{GB}) \right) \cdot (1-p^{p}_{GB}-p^{p}_{BG})^{t} \Big]\\
&>\Delta w s_{0} \Big[ (p^{a}_{BG}-p^{a}_{GB})-(p^{p}_{BG}-p^{p}_{GB}) \\
&-\frac{(p^{a}_{BG}-p^{a}_{GB})-(p^{p}_{BG}-p^{p}_{GB})}{p^{p}_{GB}+p^{p}_{GB}} \Big]\\
&=\Delta w s_{0} \left( (p^{a}_{BG}-p^{a}_{GB})-(p^{p}_{BG}-p^{p}_{GB}) \right) \cdot \left( 1-\frac{1}{p^{p}_{GB}+p^{p}_{GB}} \right)\\
& > 0.
\end{align*}
Thus, we have proved the theorem.
% \section{MILP of \textsc{GetPeriodTable} and additional fairness constraints}
% The desired period of each district can be solved by the following Mixed Integer Linear Programing:
% \begin{algorithm}[H]
% \caption{\textsc{GetPeriodTable} }
% \begin{algorithmic}[1] %[1] enables line numbers
% \STATE $H^{u}_v(\tau_v) \gets \frac{1}{\tau_v}\mathbf{\bar{b}^{u}_v}\mathbf{P}^{*}_v(\tau_v,\pi^{u})\mathbf{n}_{v,G}$ $\forall v \in V$, $\forall t \in \{1,2...T\}$
% \STATE Add $|V| \times |T|$ binary variables $x_{v,t} \in \{0,1\}$
% \STATE $\sum_{v} x_{v,t} \leq 1$ \textit{//Add constraints of periods}
% \STATE $\sum_{v} \frac{x_v}{\tau_v} \leq k$ \textit{//Add budget constraints}
% \STATE $R \leq x_{v,\tau} H^{u}_v(\tau_v)$ \textit{//Add reward}
% \STATE Solve the MILP by maximize $R$
% \RETURN $\{\tau_1,\tau_2,\dots \tau_v \dots \tau_m \}$ s.t. $x_{v,\tau}=1$ 
% \end{algorithmic}
% \end{algorithm}
% Further more, some fairness constraints can easily be realized by adjusting the MILP. We list a few examples here:
% \begin{itemize}
% \item Minimum visiting frequency fmin=1/Tmin: Replace T with smaller Tmin.
% \item Minimum individual selection fraction (with network effect):  Add constraints$\sum_{u\in V}\frac{w_{u,v}}{\tau_u} \geq L \forall v\in V$ to the MILP.
% \item Minimum individual expected utility: Replace the reward with the welfare function $R \leq x_{v,\tau} (\frac{H^{u}_v(\tau_v)}{n_v})^{\alpha}/\alpha$
% for $\alpha\leq 1$.
% \end{itemize}

%\section{Sensitivity analysis against graph perturbations.}
